# Supplementary material for: Defining the prime numbers prior to the integers: A first-principles approach to the distribution of primes
Source: arXiv:1808.09447 ancillary file (2018-08-28)
Supplement: Supplementary file 1 [file structure_of_primes_arXiv_2018_supp_mat.pdf]

# SUPPLEMENTARY INFORMATION: "DEFINING THE PRIME NUMBERS PRIOR TO THE INTEGERS: A FIRST-PRINCIPLES APPROACH TO THE DISTRIBUTION OF PRIMES"

KOLBJØRN TUNSTRØM

## 1. Materials and methods

All numerical investigations and the production of figures were performed with the mathematical software Mathematica (v10.4.1.0).

## 2. Standard notation

From the perspective of standard number theory, it is reasonable to say that what we are promoting is a coprime-view of the primes. In this context, it is natural to express $\rho_i(n)$ in terms the greatest common divisor function $(n, p_i)$, which equals 1 whenever $n$ and $p_i$ are coprime, and $p_i$ otherwise. The prime counting function $\pi(x)$ can then be written on the form

$$\pi(x) = \sum_{\substack{n \leq x \\ (n, P(\sqrt{n}))=1}} 1 - 1 \sim \frac{x}{\log x},$$

where $P(x)$ is the product of all primes less or equal to $x$. We now construct the RM in terms of

$$\pi_{\mathrm{RM}}(x) = \sum_{\substack{n \leq x \\ (n+a, P(\sqrt{n}))=1}} 1 - 1 \sim 2\mathrm{e}^{-\gamma} \frac{x}{\log x},$$

where $a$ is a random integer defined so that $a \equiv b_k \pmod{p_k}$ with probability $1/p_k$ for all $b_k \in \{0, 1, \ldots, p_k - 1\}$ and $0 \leq k \leq \pi(\sqrt{n})$. Thus, $(n + a, P(\sqrt{n}))$ can take any admissible value from 1 to $P(\sqrt{n})$. The $\mathrm{RM}_c$ in turn can be expressed as

$$\pi_{\mathrm{RM}_c}(x) = \sum_{\substack{n \leq x \\ (n+a, P(\sqrt{n}))=1}} 1 - 1,$$

restricted to those values of $a$ such that $(n + a, P(\sqrt{n})) \leq n$ for all $n \leq x$.

## 3. Asymptotic mean of $\mathrm{RM}_c$

We here present a proof of Proposition 3.2 in the main text. The proof was provided by the user Lucia at the website MathOverflow and have been published online [1]. As mentioned there, the proof follows ideas of Dress, Iwaniec and Tenenbaum [2] and further details in a related calculation can be found in their work. The proof below is only a slight rearrangement of the proof given in [1], and as Lucia states there, the argument outlined is a quick sketch, and some details would need to be filled in.

**Proposition S3.1.** *[Proposition 3.2 main text] The sum* $\sum_{\substack{d|P(\sqrt{x})\\ d\le x}} \frac{\mu(d)}{d}$ *satisfies the asymptotic relation*

$$\sum_{\substack{d|P(\sqrt{x})\\ d\le x}} \frac{\mu(d)}{d} \sim \frac{1}{\log x}.$$

*Proof.* First, put

$$S(x) = \sum_{\substack{d|P(\sqrt{x})\\ d\le x}} \frac{\mu(d)}{d} \quad \text{and} \quad M(x) = \sum_{n\le x} \frac{\mu(n)}{n}.$$

Note that $S(x)$ counts all $n \le x$ except for those $n$ having a prime factor $p$ larger than $\sqrt{x}$. Thus

$$S(x) = M(x) - \sum_{p>\sqrt{x}} \sum_{\substack{n\le x\\ p|n}} \frac{\mu(n)}{n}.$$

By the prime number theorem $M(x) = O((\log x)^{-A})$ for any $A > 0$ and $x$ large enough, and so we focus just on the second term above. Writing $n = mp$ this is

$$\sum_{p>\sqrt{x}} \frac{1}{p} \sum_{m\le x/p} \frac{\mu(m)}{m}.$$

Now let $1 \le k \le \sqrt{x}$ and group the primes $p$ above according to the ranges $x/(k+1) < p \le x/k$. Thus the sum above equals

$$\sum_{1\le k\le\sqrt{x}} M(k) \sum_{x/(k+1)<p\le x/k} \frac{1}{p}.$$

Now use the asymptotics for the sum of the reciprocals of primes to see that the inner sum over $p$ above is

$$\sim \log \frac{\log(x/k)}{\log(x/(k+1))} \sim \frac{\log(1+1/k)}{\log x}.$$

From this we obtain the asymptotic

$$S(x) \sim \frac{1}{\log x} \sum_{k=1}^{\infty} M(k) \log\Big(1 + \frac{1}{k}\Big),$$

where the bound on $M(k)$ guarantees that the sum above is convergent. To compute this constant, note that

$$\sum_{k=1}^{K} M(k)\log\left(1+\frac{1}{k}\right) = \sum_{n\le K}\frac{\mu(n)}{n}\sum_{k=n}^{K}\log(1+1/k) = \sum_{n\le K}\frac{\mu(n)}{n}\log\frac{K+1}{n}.$$

Since $\sum_{n=1}^{K}\mu(n)/n = O((\log K)^{-A})$ and $-\sum_{n=1}^{\infty}\mu(n)(\log n)/n = 1$, it follows that the constant is in fact 1, and hence that $S(x)\sim 1/\log x$.

□

## 4. Covariance expression

In an elementary calculation, Hausman and Shapiro [4] derived the variance of the number of reduced residues modulo $n$ in an arbitrary interval of length $h$. We here extend to the general case of the covariance between two intervals $A_1$ and $A_2$ with corresponding lengths $h_1$ and $h_2$ that are separated by a distance $q$, and where in $A_1$ we regard the number of reduced residues modulo $n_1$, and in $A_2$ the number of reduced residues modulo $n_2$. The resulting expressions for the covariance we present here follows from a straight forward adaption of Hausman and Shapiro's proof.

To begin, let

$$f_n(m) := \begin{cases} 1 & \text{if} \quad (m,n) = 1, \\ 0 & \text{if} \quad (m,n) > 1. \end{cases}$$

The function of $f_n(m)$ is to weed out coprimes to $n$. To count the number of such in the integer set $A_m^h := \{m+i\}_{i=0}^{h-1}$, we define

$$F_n(m,h) := \sum_{j=m}^{m+h-1} f_n(j).$$

Suppose now the two integer sets $A_m^{h_1}$ and $A_{m+q}^{h_2}$ of lengths $h_1$ and $h_2$ and that are separated by a distance $q$. In $A_m^{h_1}$ we consider the number of reduced residues modulo $n_1$, $F_{n_1}(m,h_1)$; in $A_{m+q}^{h_2}$ we consider the number of reduced residues modulo $n_2$, $F_{n_2}(m+q,h_2)$. The covariance between $F_{n_1}(m,h_1)$ and $F_{n_2}(m+q,h_2)$ is given by

$$G(n_1,n_2,h_1,h_2,q) := \frac{1}{n_1 n_2} \sum_{m=1}^{n_1 n_2} F_{n_1}(m,h_1) F_{n_2}(m+q,h_2) - h_1 h_2 \frac{\phi(n_1)\phi(n_2)}{n_1 n_2},$$

where $\phi(n)$ is Euler's totient function.

For brevity, we consider the case when $h_2 \geq h_1$ and $n_1$ and $n_2$ are both even. Similar expressions can be derived in the other cases. Under this assumption, and introducing the abbreviation

$$Q(n_1,n_2) := \frac{1}{2} \prod_{p \mid \left(n_1 n_2/(n_1,n_2)^2\right)} \left(1 - \frac{1}{p}\right) \prod_{p \mid (n_1,n_2)'} \left(1 - \frac{2}{p}\right),$$

where $(n_1, n_2)$ denotes the greatest common divisor of $n_1$ and $n_2$ and $n'$ denotes the largest odd divisor of $n$, we have that

$$\frac{1}{n_1 n_2}\sum_{m=1}^{n_1 n_2} F_{n_1}(m,h_1)F_{n_2}(m+q,h_2) =$$

$$Q(n_1,n_2)\sum_{\substack{k=1\\2|q+k-1}}^{h_2-h_1+1} h_1 \prod_{\substack{p|(n_1,n_2)'\\p|(q+k-1)}}\left(1+\frac{1}{p-2}\right)+$$

$$Q(n_1,n_2)\sum_{\substack{k=1\\2|(q+h_2-h_1+k)}}^{h_1-1}(h_1-k)\prod_{\substack{p|(n_1,n_2)'\\p|(q+h_2-h_1+k)}}\left(1+\frac{1}{p-2}\right)+$$

$$Q(n_1,n_2)\sum_{\substack{k=1\\2|(q-k)}}^{h_1-1}(h_1-k)\prod_{\substack{p|(n_1,n_2)'\\p|(q-k)}}\left(1+\frac{1}{p-2}\right).$$

Both the numerical and theoretical results presented in this inquiry are obtained from this expression. It is possible, however, to derive a more compact theoretical expression in terms of the Möbius function

$$\mu(d) := \begin{cases} 1 & \text{if } d = 1, \\ (-1)^k & \text{if } d \text{ is a product of } k \text{ distinct primes,} \\ 0 & \text{if } d \text{ has one or more repeated prime factors.} \end{cases}$$

In order to achieve this, we also need the following set of definitions:

**Definitions.** For any square-free integer $n$,

$$\rho(n) := \prod_{p|n}(p-2);$$

$$\gamma^+(h,q,d) := \begin{cases} 0 & \text{if } d \nmid q+i \text{ for all } i, \text{ where } 1 \le i \le d\left\{\frac{h}{d}\right\}, \\ 1 & \text{if } d \mid q+i \text{ for some } i, \text{ where } 1 \le i \le d\left\{\frac{h}{d}\right\}; \end{cases}$$

$$\gamma^-(h,q,d) := \begin{cases} 0 & \text{if } d \nmid q-i \text{ for all } i, \text{ where } 1 \le i \le d\left\{\frac{h}{d}\right\}, \\ 1 & \text{if } d \mid q-i \text{ for some } i, \text{ where } 1 \le i \le d\left\{\frac{h}{d}\right\}; \end{cases}$$

and

$$\left\{\frac{q}{d}\right\}_1 := \begin{cases} \left\{\frac{q}{d}\right\} & \text{if } d \nmid q, \\ 1 & \text{if } d \mid q. \end{cases}$$

Then we can write the covariance $G(n_1, n_2, h_1, h_2, q)$ on the equivalent form

$$G(n_1,n_2,h_1,h_2,q) = \frac{1}{n_1 n_2}Q(n_1,n_2)\sum_{d|(n_1,n_2)'}\frac{\mu^2(d)}{\rho(d)}\mathcal{B}(h_1,h_2,q,d),$$

where

$$\begin{aligned}
&\mathcal{B}(h_1,h_2,q,d)\\
&\quad = h_1\left(\frac{1}{2d}-\left\{\frac{h_2-h_1+1}{2d}\right\}+\left\{\frac{q+h_2-h_1}{2d}\right\}-\left\{\frac{q}{2d}\right\}_1\right)\\
&\quad - 2d\left\{\frac{h_1}{2d}\right\}\left(\left\{\frac{h_1}{2d}\right\}+\left\{\frac{q+h_2-h_1}{2d}\right\}-\left\{\frac{q}{2d}\right\}_1\right)\\
&\quad + \gamma^+(h_2-h_1+1,q-1,2d)h_1\\
&\quad + \gamma^+(h_1,q+h_2-h_1,2d)2d\left(\left\{\frac{h_1}{2d}\right\}-\left(1-\left\{\frac{q+h_2-h_1}{2d}\right\}\right)\right)\\
&\quad + \gamma^-(h_1,q,2d)2d\left(\left\{\frac{h_1}{2d}\right\}-\left\{\frac{q}{2d}\right\}_1\right).
\end{aligned}$$

Numerical investigations hint to a possible simplification of this expression, as some of the terms appear to always cancel each other, but this remains to be shown theoretically. Whenever $A_1 = A_2$, so that $h_1 = h_2 = h$ and $n_1 = n_2 = n$, we can write $H(n,h) := G(n,n,h,h,0)$, and obtain to the variance derived in [4],

$$H(n,h) = \prod_{p|n'}\left(1-\frac{2}{p}\right)\sum_{d|n'}\frac{\mu^2(d)}{\rho(d)}d\left\{\frac{h}{2d}\right\}\left(1-\left\{\frac{h}{2d}\right\}\right).$$

4.1. **Application to the RM.** In terms of the variance function $H(n,h)$ and the covariance function $G(n1,n2,h1,h2,q)$, the variance of $\pi_{\mathrm{RM}}(x)$ can be expressed as

$$\begin{aligned}
\mathrm{Var}(\pi_{\mathrm{RM}}(x)) &= \sum_{i=1}^{[x]}\mathrm{Var}(\mathbf{1}_{\mathcal{P}_{\mathrm{RM}}}(i)^2) + 2\sum_{i=1}^{[x]}\sum_{i<j}^{[x]}\mathrm{Cov}\left(\mathbf{1}_{\mathcal{P}_{\mathrm{RM}}}(i),\mathbf{1}_{\mathcal{P}_{\mathrm{RM}}}(j)\right)\\
&= \sum_{i=1}^{[x]} H(P(\sqrt{i}),1) + 2\sum_{i=1}^{[x]}\sum_{i<j}^{[x]} G(P(\sqrt{i}),P(\sqrt{j}),1,1,j-i),
\end{aligned}$$

where $P(x)$ is defined as the product of all primes less or equal to $x$.

4.2. **Propositions.** We here provide proofs for two of the propositions in the paper, 3.4 and 3.5 respectively.

**Proposition S4.1.** *[Proposition 3.4 main text] The covariance* $\mathrm{Cov}\left(\mathbf{1}_{\mathcal{P}_{\mathrm{RM}}}(i),\mathbf{1}_{\mathcal{P}_{\mathrm{RM}}}(j)\right)$ *satisfies the relation*

$$\sum_{i<j}^{[x]}\mathrm{Cov}\left(\mathbf{1}_{\mathcal{P}_{\mathrm{RM}}}(i),\mathbf{1}_{\mathcal{P}_{\mathrm{RM}}}(j)\right) \le 0,$$

*where the inequality is strict for* $i \ge 25$.

*Proof.* Let us first rewrite the covariance sum as

$$\sum_{i<j}^{[x]}\mathrm{Cov}\left(\mathbf{1}_{\mathcal{P}_{\mathrm{RM}}}(i),\mathbf{1}_{\mathcal{P}_{\mathrm{RM}}}(j)\right) = \sum_{j=1}^{n} G\left(P(\sqrt{i}),P(\sqrt{i+j}),1,1,j\right).$$

Here we have replaced $[x] - i$ by $n$, and $P(x)$ is the product of all primes less or equal to $x$. Consider now the sum

$$S(q) = \sum_{j=1}^{n} G\left(P(\sqrt{i}), P(\sqrt{i+j}), 1, 1, j+q\right).$$

This function is periodic in $q$ with period $P(\sqrt{i})$ and also satisfies $\sum_{q=0}^{P(\sqrt{i})-1} S(q) = 0$. Hence, there must be values of $q$ such that $S(q) \leq 0$. To prove the proposition we want to show that $q = 0$ is one such value.

To show that some value $\overline{q}$ satisfies $S(\overline{q}) \leq 0$, it suffices to show that it is a minimum value, that is, $S(\overline{q}) \leq S(q)$ for $0 \leq q \leq P(\sqrt{i})$. To proceed, we write $S(q)$ as

$$\begin{aligned} S(q) &= \sum_{j=1}^{n} G\left(P(\sqrt{i}), P(\sqrt{i+j}), 1, 1, j+q\right) \\ &= \sum_{\substack{j=1 \\ 2|j+q}}^{n} \frac{1}{2} \prod_{p|\frac{P(\sqrt{i+j})}{P(\sqrt{i})}} \left(1 - \frac{1}{p}\right) \prod_{p|\frac{P(\sqrt{i+j})}{2}} \left(1 - \frac{2}{p}\right) \prod_{\substack{p|\frac{P(\sqrt{i+j})}{2} \\ p|j+q}} \left(1 + \frac{1}{p-2}\right) \\ &\quad - \sum_{j=1}^{n} \prod_{p|P(\sqrt{i})} \left(1 - \frac{1}{p}\right) \prod_{p|P(\sqrt{i+j})} \left(1 - \frac{1}{p}\right). \end{aligned}$$

Note that after the final equality the last term is constant and not affected by the choice of $q$, while the first term is always positive. We therefore need to find $q$ such that this term is minimised. Continuing, we rewrite the term as

$$\begin{aligned} &\sum_{\substack{j=1 \\ 2|j+q}}^{n} \frac{1}{2} \prod_{p|\frac{P(\sqrt{i+j})}{P(\sqrt{i})}} \left(1 - \frac{1}{p}\right) \prod_{p|\frac{P(\sqrt{i+j})}{2}} \left(1 - \frac{2}{p}\right) \prod_{\substack{p|\frac{P(\sqrt{i+j})}{2} \\ p|j+q}} \left(1 + \frac{1}{p-2}\right) \\ &= \frac{1}{2} \prod_{p|P(\sqrt{i})} \left(1 - \frac{1}{p}\right)^{-1} \prod_{p|\frac{P(\sqrt{i})}{2}} \left(1 - \frac{2}{p}\right) \sum_{\substack{j=1 \\ 2|j+q}}^{n} \prod_{p|P(\sqrt{i+j})} \left(1 - \frac{1}{p}\right) \prod_{\substack{p|\frac{P(\sqrt{i})}{2} \\ p|j+q}} \left(1 + \frac{1}{p-2}\right). \end{aligned}$$

The two products before the sum are both constant, so our problem reduces to that of finding a $q$ that minimises the sum

$$\text{(S1)} \qquad \sum_{\substack{j=1 \\ 2|j+q}}^{n} \prod_{p|P(\sqrt{i+j})} \left(1 - \frac{1}{p}\right) \prod_{\substack{p|\frac{P(\sqrt{i})}{2} \\ p|j+q}} \left(1 + \frac{1}{p-2}\right).$$

Consider for a moment the similar sum

$$\text{(S2)} \qquad \sum_{\substack{j=1 \\ 2|j+q}}^{n} \prod_{\substack{p|\frac{P(\sqrt{i})}{2} \\ p|j+q}} \left(1 + \frac{1}{p-2}\right).$$

For $n$ even, this sum has minimum values at $q = 0$ or $q = 1$, which follows from the fact that the term $\left(1 + \frac{1}{p-2}\right) > 1$ for any given value of $p > 2$, together with the fact that for each such value $p$, this term occurs exactly $\lfloor (n/2)/p \rfloor$ times across the

sum. Increasing $q$ could alter the number of occurrences to $\lfloor (n/2)/p \rfloor + 1$, which would increase the value of the sum. For $n$ odd, $q = 0$ corresponds to a minimum value of the sum, while $q = 1$ does not. The latter follows since the sum in this case contains an additional positive term.

Returning to (S1), note that the first product under the sum is monotonically decreasing for increasing $j$. Our argument for (S2) is therefore valid for (S1), with the only difference that for $n$ even, the sum is not guaranteed to be a minimum for $q = 1$. It follows that $S(0) \leq S(q)$ for any other value of $q$, and thus negative or 0. For the latter to be the case, that is, $S(0) = 0$, the criteria that must be fulfilled are $n = P(\sqrt{i})$ and $P(\sqrt{i+1}) = P(\sqrt{i+j})$ for $1 \leq j \leq n$. These can never hold simultanously for any values of $i \geq 25$, and in that case, $S(0) < 0$. □

**Proposition S4.2.** *[Proposition 3.5 main text] Let* $\mathrm{Corr}[x, y]$ *be the correlation function between two variables* $x$ *and* $y$*. Then we have that the RM in terms of the indicator function* $\mathbf{1}_{\mathcal{P}_{\mathrm{RM}}}(m)$ *satisfies the relation*

$$\lim_{m,n\to\infty} \mathrm{Corr}[\mathbf{1}_{\mathcal{P}_{\mathrm{RM}}}(m), \mathbf{1}_{\mathcal{P}_{\mathrm{RM}}}(n)] = 0,$$

*for any fixed distance* $n - m > 0$*.*

*Proof.* From the derived expressions for $H$ and $G$, the correlation function $\mathrm{Corr}[\mathbf{1}_{\mathcal{P}_{\mathrm{RM}}}(m), \mathbf{1}_{\mathcal{P}_{\mathrm{RM}}}(n)]$ can be rewritten as

$$\mathrm{Corr}[\mathbf{1}_{\mathcal{P}_{\mathrm{RM}}}(m), \mathbf{1}_{\mathcal{P}_{\mathrm{RM}}}(n)] = \frac{G(P(\sqrt{m}), P(\sqrt{n}), 1, 1, n-m)}{\sqrt{H(P(\sqrt{m}), 1)}\sqrt{H(P(\sqrt{n}), 1)}} =$$

$$\frac{\prod_{p|P(\sqrt{n})/P(\sqrt{m})} \sqrt{\left(1 - \frac{1}{p}\right)} \prod_{\substack{p|P(\sqrt{m}) \\ p\nmid n-m}} \left(1 - \frac{1}{p-1}\right) - \prod_{p|P(\sqrt{m})} \sqrt{\left(1 - \frac{1}{p}\right)} \prod_{p|P(\sqrt{n})} \sqrt{\left(1 - \frac{1}{p}\right)}}{\sqrt{\left(1 - \prod_{p|P(\sqrt{m})} \left(1 - \frac{1}{p}\right)\right)\left(1 - \prod_{p|P(\sqrt{n})} \left(1 - \frac{1}{p}\right)\right)}}.$$

It is straightforward to see that for any fixed $n - m > 0$, the numerator converges to 0 as $m, n \to \infty$, while the denominator converges to 1, which completes the proof. □

## 5. Tables

Table S1. Size of sample spaces of the counting functions $\pi_{\mathrm{RM}_c}(x)$ and $\pi_{\mathrm{RM}}(x)$ for different values of $x = p_{k+1}^2 - 1$, $0 \leq k \leq 45$. For $\pi_{\mathrm{RM}}(x)$, the exact size of the sample space for each value of $k$ is given by $\prod_{i=1}^{k} p_i$. The values in the third column are numerically rounded approximations to these values for $k > 7$.

| $k$ | # samples $\pi_{\mathrm{RM}_c}(x)$ | # samples $\pi_{\mathrm{RM}}(x)$ |
|---|---|---|
| 0 | 1 | 1 |
| 1 | 2 | 2 |
| 2 | 6 | 6 |
| 3 | 25 | 30 |
| 4 | 53 | 210 |
| 5 | 234 | 2310 |
| 6 | 97 | 30030 |
| 7 | 262 | 510510 |
| 8 | 159 | $9.70 \times 10^{6}$ |
| 9 | 63 | $2.23 \times 10^{8}$ |
| 10 | 392 | $6.47 \times 10^{9}$ |
| 11 | 44 | $2.01 \times 10^{11}$ |
| 12 | 151 | $7.42 \times 10^{12}$ |
| 13 | 487 | $3.04 \times 10^{14}$ |
| 14 | 106 | $1.31 \times 10^{16}$ |
| 15 | 88 | $6.15 \times 10^{17}$ |
| 16 | 65 | $3.26 \times 10^{19}$ |
| 17 | 757 | $1.92 \times 10^{21}$ |
| 18 | 55 | $1.17 \times 10^{23}$ |
| 19 | 216 | $7.86 \times 10^{24}$ |
| 20 | 972 | $5.58 \times 10^{26}$ |
| 21 | 63 | $4.07 \times 10^{28}$ |
| 22 | 163 | $3.22 \times 10^{30}$ |
| 23 | 88 | $2.67 \times 10^{32}$ |
| 24 | 115 | $2.38 \times 10^{34}$ |
| 25 | 440 | $2.31 \times 10^{36}$ |
| 26 | 5236 | $2.33 \times 10^{38}$ |
| 27 | 512 | $2.40 \times 10^{40}$ |
| 28 | 5683 | $2.57 \times 10^{42}$ |
| 29 | 598 | $2.80 \times 10^{44}$ |
| 30 | 44 | $3.16 \times 10^{46}$ |
| 31 | 231 | $4.01 \times 10^{48}$ |
| 32 | 88 | $5.26 \times 10^{50}$ |
| 33 | 1533 | $7.20 \times 10^{52}$ |
| 34 | 44 | $1.00 \times 10^{55}$ |
| 35 | 1873 | $1.49 \times 10^{57}$ |
| 36 | 176 | $2.25 \times 10^{59}$ |
| 37 | 264 | $3.54 \times 10^{61}$ |
| 38 | 482 | $5.77 \times 10^{63}$ |
| 39 | 88 | $9.63 \times 10^{65}$ |
| 40 | 88 | $1.67 \times 10^{68}$ |
| 41 | 2443 | $2.98 \times 10^{70}$ |
| 42 | 44 | $5.40 \times 10^{72}$ |
| 43 | 2455 | $1.03 \times 10^{75}$ |
| 44 | 2108 | $1.99 \times 10^{77}$ |
| 45 | 23759 | $3.92 \times 10^{79}$ |

## 6. Figures

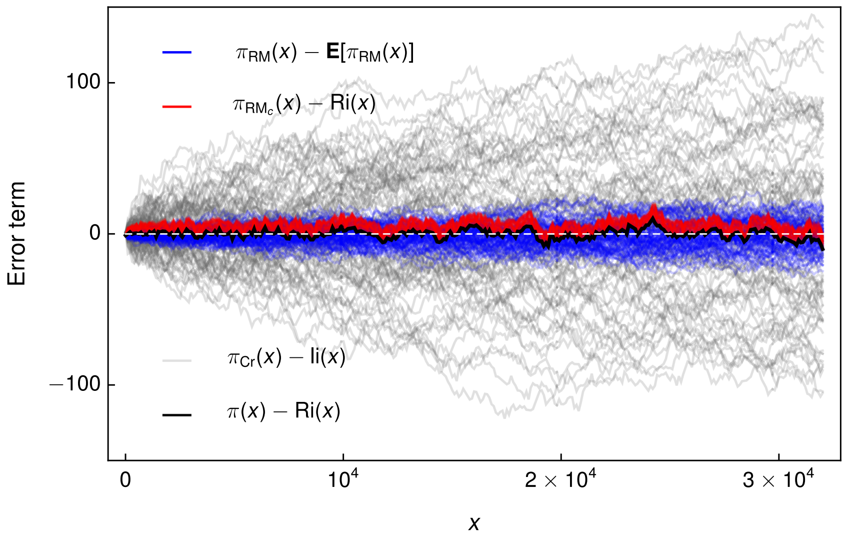


Figure S1. Comparing Cramer's random model with the RM and the $\mathrm{RM}_c$. Cramer's random model can be defined in terms of $n$ being a "prime" with probability $1/\log n$ for $n > 2$. We count the "primes" below $x$ in this case by the counting function $\pi_{\mathrm{Cr}}(x)$, which has expected value equal to $\sum_{n=3}^{[x]} 1/\log n \sim \mathrm{li}(x)$. In the figure we see 88 realisations of $\pi_{\mathrm{Cr}}(x) - \mathrm{li}(x)$ (gray), together with 88 realisations of $\pi_{\mathrm{RM}}(x) - \mathbf{E}[\pi_{\mathrm{RM}}(x)]$ (blue), and all 88 realisations of $\pi_{\mathrm{RM}_c}(x) - \mathrm{Ri}(x)$ present at $x = p_{41}^2 - 1$ (red), which includes the primes, $\pi(x) - \mathrm{Ri}(x)$ (black). Here $\mathrm{Ri}(x)$ is the Riemann function defined in section 3a in the main text. In particular, we observe that the RM is subrandom, having variance smaller than that of Cramer's random model. Since the RM is constructed on the structure of the primes, it does a much better job at capturing the fluctuating behaviour of $\pi(x)$. The realisations of the $\mathrm{RM}_c$ lie in a constrained subspace of the RM, are strongly correlated, and display even smaller variance than the RM.

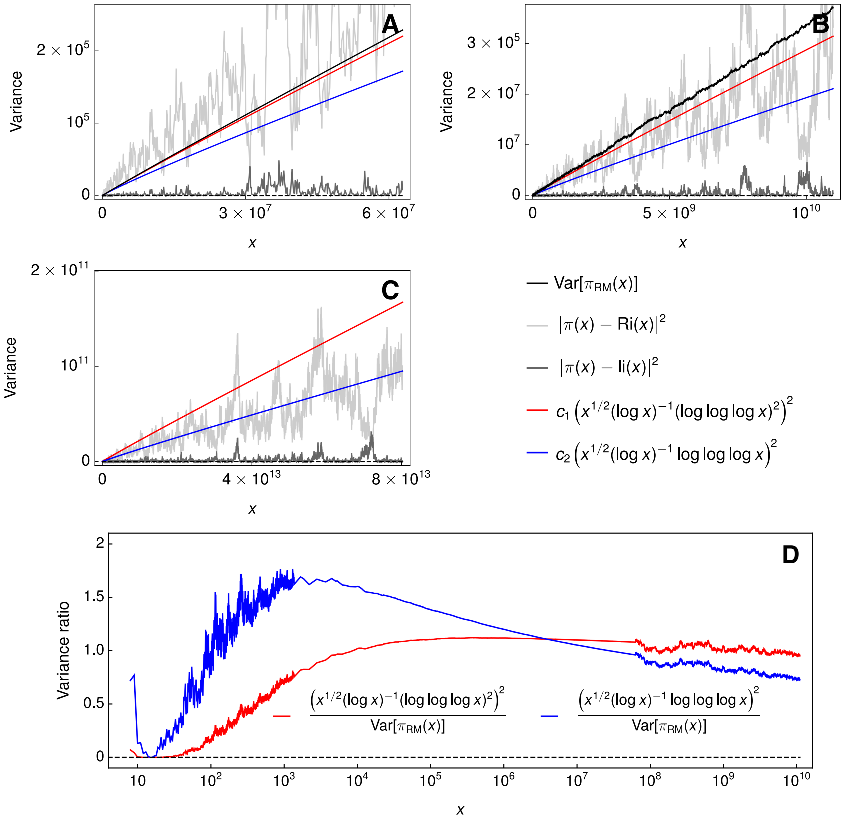


Figure S2. Comparison of $\mathrm{Var}[\pi_{\mathrm{RM}}(x)]$ with the error terms $|\pi(x) - \mathrm{Ri}(x)|^2$ and $|\pi(x) - \mathrm{li}(x)|^2$. In order to predict long term behaviour, the comparison includes the estimates from Littlewood's omega result [3, p. 479], $\pi(x) - \mathrm{li}(x) = \Omega_{\pm}\left(x^{1/2}(\log x)^{-1} \log\log\log x\right)$ and Monach and Montgomery's conjecture [3, p. 484], $\pi(x) - \mathrm{li}(x) = O\left(x^{1/2}(\log x)^{-1}(\log\log\log x)^2\right)$. A, B, and C shows the different terms plotted against $x = p_{k+1}^2 - 1$, with $k_{max}$ equal to $10^3$, $10^4$, and $6 \times 10^5$, respectively. In A, data for $\mathrm{Var}[\pi_{\mathrm{RM}}(x)]$ are theoretically computed, while in B, estimated as the average of $|\pi_{\mathrm{RM}}(x) - \mathbf{E}[\pi_{\mathrm{RM}}(x)]|^2$ over 1000 realisations of the RM. Similar data is not available in C. In D, we see the ratios of the two theoretical estimates to $\mathrm{Var}[\pi_{\mathrm{RM}}(x)]$. For $4 \le x < 1369$, data is plotted at every $[x]$, beyond this at $x = p_{k+1}^2 - 1$, $12 \le k \le 10^4$. Data for $x < p_{1001}^2$ are theoretically computed, the remaining data are estimated as stated above. Both curves in D appear to reach a peak before declining, indicating that $\mathrm{Var}[\pi_{\mathrm{RM}}(x)]$ grows asymptotically faster than both theoretical estimates. How fast awaits theoretical investigation. The maximum value of the red curve is reached at around $x = p_{111}^2 - 1 = 368448$. To obtain a consistent comparison of growths in A, B, and C, we have normalised the two estimates by $c_1$ and $c_2$, defined so that the normalised estimates equal $\mathrm{Var}[\pi_{\mathrm{RM}}(x)]$ at this value of $x$. While $\mathrm{Var}[\pi_{\mathrm{RM}}(x)]$ lies well above $|\pi(x) - \mathrm{Ri}(x)|^2$ in both A and B, the same is not true for $|\pi(x) - \mathrm{li}(x)|^2$. But we do see the tendency in B of $\mathrm{Var}[\pi_{\mathrm{RM}}(x)]$ overcoming $|\pi(x) - \mathrm{li}(x)|^2$. Given the observed asymptotic growth of $\mathrm{Var}[\pi_{\mathrm{RM}}(x)]$ and Monach and Montgomery's conjecture, we should expect this trend to continue—as it seemingly does in C—so that $\mathrm{Var}[\pi_{\mathrm{RM}}(x)]$ eventually becomes strictly larger than $|\pi(x) - \mathrm{li}(x)|^2$. If $|\pi(x) - \mathrm{li}(x)|^2$ accurately estimates $\mathbf{E}[|\pi_{\mathrm{RM}_c}(x) - \mathrm{li}(x)|^2]$, as suggested in the main text, we have here that the variance of the RM grows faster than that of the $\mathrm{RM}_c$, an anticipated consequence of the strong constraint put on the elements in the $\mathrm{RM}_c$.

## References

[1] Lucia. Asymptotic limit of truncated legendre sieve. MathOverflow, 2015. URL (version: 2017-04-03): http://mathoverflow.net/q/203659.

[2] Dress, F, Iwaniec, H, Tenenbaum, G (1983) Sur une somme liée à la fonction de Möbius. *Journal für die reine und angewandte Mathematik* 340:53–58

[3] Montgomery HL, Vaughan RC (2007) *Multiplicative number theory. I. Classical theory*, Cambridge Studies in Advanced Mathematics. (Cambridge University Press, Cambridge) Vol. 97.

[4] Hausman M, Shapiro HN (1973) On the mean square distribution of primitive roots of unity. *Commun Pure App Math* 26:539–547.

*E-mail address*: kolbjorn@chalmers.se

Department of Physics, Chalmers University of Technology, 41296 Gothenburg, Sweden
